# Supplementary material for: Does On-Policy Distillation Need to Complete Every Rollout?
Source: arXiv:2610.21337 source file (2026-11-17)
Supplement: Supplementary file 1 [file appendix_tir.tex]

% TIR extension, audited against sOPD origin/tir ad7a32c (2026-10-16).
% Data: results/tir-s4t30/data/{evals.json,series/*.json}.
\clearpage
\section{Tool-Integrated Reasoning}
\label{app:tir}

We evaluate \method{} on mathematics with a Python interpreter, where student-generated reasoning and tool calls alternate with interpreter observations. We compare \method{} with Vanilla OPD over three paired training seeds.

\subsection{Setup and Extension to Tool Observations}
\label{app:tir-setup}

We distill Qwen3-30B-A3B-Instruct-2507 into Qwen3-4B in non-thinking mode on 14{,}393 filtered Nemotron-Cascade-RL-Math problems. Each response allows up to 16 assistant turns. Python executes in a stateless subprocess with a 30-second timeout, and observations are limited to 5{,}000 characters.

Training follows Section~\ref{sec:experimental-setup}, with batch size $B=256$, AdamW at learning rate $10^{-6}$, and block width $K=128$. The response cap $L=16{,}384$ includes tool observations. Both methods continue the model and optimizer state of a shared 25-step Vanilla warmup to step 200. Each arm uses two NVIDIA H20 GPUs, with both arms of each seed on the same host.

\paragraph{Position counting and loss masking.}
We sample the stopping position before the entire rollout using Eq.~\eqref{eq:stop}. Positions count both student tokens and tool observations, but only student tokens contribute to the loss. An observation that would reach or exceed the remaining budget is dropped in full, and the rollout stops. On the capped full trajectory, let $m_{i,t}$ indicate a student token at response position $t$, and let $I_{i,t}=\ind\{S_i\geq t\}$ be the cutoff indicator. With the inclusion probability $p_t$ in Eq.~\eqref{eq:survival}, the estimators become
\begin{equation}
\widehat G_k=\sum_{i,t}\frac{I_{i,t}m_{i,t}}{p_t}h_{i,t},
\qquad
\widehat N_k=\sum_{i,t}\frac{I_{i,t}m_{i,t}}{p_t}.
\label{eq:tir-masked-ipw}
\end{equation}
Under prefix-local token losses and a prefix-conditioned tool-response distribution independent of the sampled cutoff, Appendix~\ref{app:preservation} applies to student tokens: $\widehat G_k$ preserves their capped full gradient sum in expectation. We use $C_{26}=N_{25}$ and then $C_k=\widehat N_{k-1}$ as in Eq.~\eqref{eq:lagged}. The normalized estimator therefore targets $G_k/C_k$, rather than the full-batch token mean.

\paragraph{Evaluation.}
We evaluate the same TIR-trained checkpoints with and without the interpreter, using the five mathematics benchmarks and sampling settings of Section~\ref{sec:experimental-setup}. The 32{,}768-position evaluation budget includes observations when tools are enabled. We evaluate every 25 steps with the interpreter, and at steps 25, 50, 100, 150, and 200 without it. Accuracy is the unweighted mean of the five benchmark scores. Figures show the mean and range over three seeds; the accuracy table reports the mean and sample standard deviation.

\subsection{Accuracy at Matched Steps and Training Time}
\label{app:tir-accuracy}

Figure~\ref{fig:tir} shows that \method{} and Vanilla follow similar accuracy trends, with values at each checkpoint in Table~\ref{tab:results-tir}. Across the seven post-warmup checkpoints with tools, the \method{}--Vanilla difference ranges from $-1.15$ to $+0.62$ percentage points. At step 200, \method{} reaches $59.2$ with the interpreter and $59.0$ without it, compared with $60.0$ and $58.5$ for Vanilla. Figure~\ref{fig:bench-tir} breaks down tool-enabled accuracy by benchmark.

\clearpage
\begin{figure}[htbp]
\centering
\includegraphics[width=0.88\textwidth]{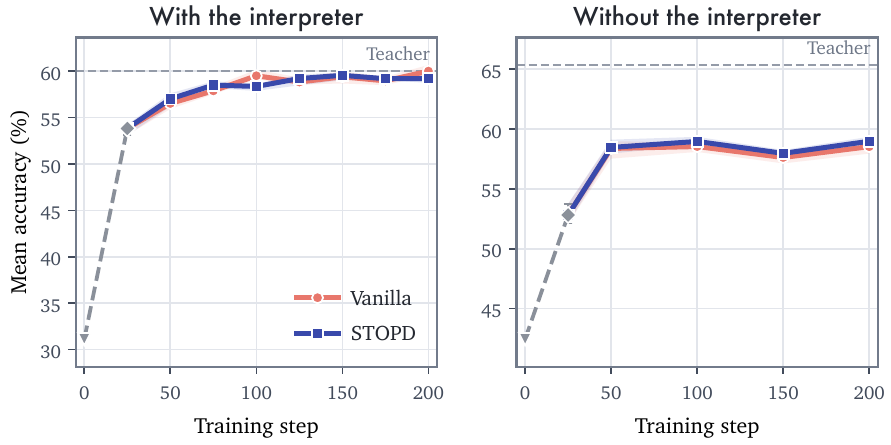}
\caption{Accuracy against training step in tool-integrated reasoning, evaluated with the interpreter (left) and without it (right). The initial student and shared warmup are gray; dashed horizontal lines show the teacher.}
\label{fig:tir}
\end{figure}

\begin{table}[htbp]
\centering
\caption{Accuracy (\%) in tool-integrated reasoning, mean $\pm$ standard deviation. Step 25 is shared warmup; initial student and teacher are fixed model evaluations. Dashes mark checkpoints not evaluated without the interpreter.}
\label{tab:results-tir}
\small
\setlength{\tabcolsep}{9pt}
\input{figs/tab_results_tir.tex}
\end{table}

Figure~\ref{fig:tir-time} plots accuracy against training time after warmup. Both methods approach the tool-enabled teacher's score of $60.0$, making threshold-based speedups sensitive to small accuracy differences. We therefore compare training time over all 175 post-warmup updates.

\begin{figure}[htbp]
\centering
\includegraphics[width=0.88\textwidth]{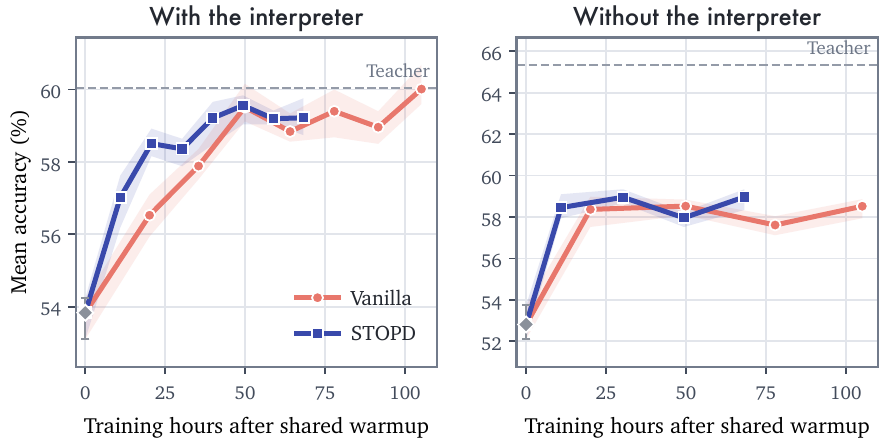}
\caption{Accuracy against training hours after the shared warmup, with mean elapsed time across seeds. Dashed lines show the teacher. Training time includes checkpoint writing and excludes evaluation.}
\label{fig:tir-time}
\end{figure}

\newpage
\subsection{Efficiency and Training Dynamics}
\label{app:tir-efficiency}

Over steps 26--200, \method{} reduces generated student tokens per response from $7{,}184$ to $5{,}193$ ($27.7\%$) and mean training-step time from $36.0$ to $23.4$ minutes (Table~\ref{tab:time-tir}). The mean speedup across paired seeds is $1.54\times$, reducing the 175 post-warmup updates from $105.1$ to $68.2$ hours. Including the shared warmup, which averages $5.8$ hours, gives a $1.50\times$ speedup over all 200 steps. As Vanilla's responses shorten, the post-warmup speedup decreases from $1.84\times$ over steps 26--50 to $1.44\times$ over steps 151--200.

\begin{table}[htbp]
\centering
\caption{Cost of a TIR training step over steps 26--200. Tokens and throughput exclude observations. Generation includes tools and teacher scoring; Other includes old-log-probability computation, checkpoint writing, and weight synchronization. Ratios average Vanilla/\method{} over paired seeds, except throughput, which uses \method{}/Vanilla.}
\label{tab:time-tir}
\small
\setlength{\tabcolsep}{5pt}
\input{figs/tab_time_tir.tex}
\end{table}

Figure~\ref{fig:tir-dynamics} shows similar entropy, distillation-loss, and gradient-norm trends, with larger local fluctuations under \method{}. Using the definition in Section~\ref{sec:batch-size-math}, loss jitter over post-warmup interior steps is $1.7\%$ for Vanilla and $8.5\%$ for \method{}, averaged across seeds; gradient-norm jitter is $6.6\%$ and $13.7\%$. The mean ratio $\widehat N_k/C_k$ is $1.003$. As in Figure~\ref{fig:dynamics}, the response-length panel uses \method{}'s estimate $\widehat N_k/B$ of the complete student-token length; its observed token count appears in Table~\ref{tab:time-tir}.

\begin{figure}[htbp]
\centering
\includegraphics[width=\textwidth]{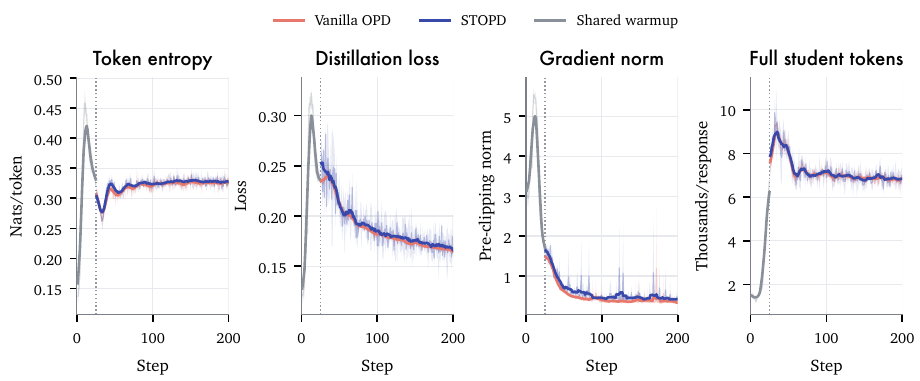}
\caption{TIR training dynamics, with shared warmup in gray. Thin curves show per-step means, thick curves a nine-step moving average, and bands the seed range. Gradient norms are measured before clipping; response length uses observed student tokens for Vanilla and estimated complete student tokens for \method{}.}
\label{fig:tir-dynamics}
\end{figure}

\FloatBarrier
\subsection{Per-Benchmark Results}
\label{app:tir-scope}

Figure~\ref{fig:bench-tir} shows that \method{} and Vanilla follow similar learning trends across the five mathematics benchmarks with the interpreter enabled. Both methods improve over the shared warmup on AIME24 and AIME25, while AMC23 and MATH500 reach closely matched final accuracy. Minerva remains near the warmup level for both methods. These per-benchmark trends complement the training-time savings in Table~\ref{tab:time-tir}, showing that \method{} maintains comparable performance while reducing training cost in this tool-enabled mathematics setting.

\begin{figure}[htbp]
\centering
\includegraphics[width=\textwidth]{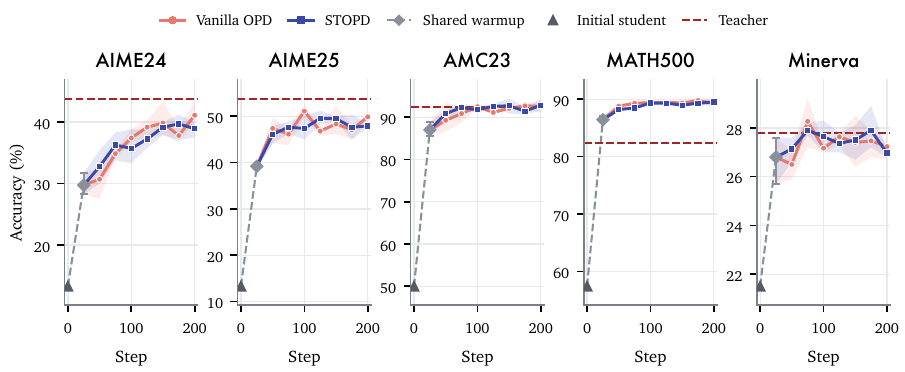}
\caption{Tool-enabled accuracy per mathematics benchmark against training step, with the initial student and shared warmup in gray.}
\label{fig:bench-tir}
\end{figure}
\clearpage
